# Supplementary material for: Mixed Monotonic Programming for Fast Global Optimization
Source: arXiv:1910.07853 source file (2020-02-27)
Supplement: Supplementary file 1 [file appendix.tex]

\section{Technical Details on the Reduction in \cref{eq:reduction:r,eq:reduction:s,eq:reduction:alpha,eq:reduction:beta}} \label{app:reduction}
The reduction must satisfy \cref{eq:alg:bb:reduction}, which is equivalent to showing that $\mathcal M \cap \mathcal D' = \mathcal M' \cap \mathcal D'$ holds with $\mathcal D'$ as defined in the convergence proof of \cref{alg:bb}. This proof is a technical extension of \cite[Lemma~11.1]{Tuy2016} and included for completeness.

Consider \cref{eq:reduction:r,eq:reduction:alpha}.
Since $r_i' = \alpha_i r_i + (1-\alpha_i) s_i$ for some $\alpha_i \in[0, 1]$, we have $r_i \le r_i' \le s_i$. Thus, $\mathcal M'\subseteq\mathcal M$ and $\mathcal M \cap \mathcal D' \supseteq \mathcal M' \cap \mathcal D'$.
For the reverse inclusion, first observe that, for every $\vec x\in\mathcal M$ and because of \cref{mmp:prop1,mmp:prop2}, $G_i(\vec x, \vec x) \le 0$ implies $G_i(\vec r, \vec x) \le 0$ and $F(\vec x, \vec x) > \gamma_k$ implies $F(\vec x, \vec r) > \gamma_k$. Hence,
$\mathcal M \cap \mathcal D' \subseteq \mathcal M \cap \bar{\mathcal D}$ with
\begin{multline}
\mathcal M \cap \bar{\mathcal D} = \{ \vec x\in\mathcal M | F(\vec x, \vec r) > \gamma_k,\\ G_i(\vec r, \vec x) \le 0 \text{ for all } i = 1, \dots, m \}.
\end{multline}

Now, any $\vec x\in\mathcal M\cap\bar{\mathcal D}$ is equal to $\vec s - \sum_{k=1}^K (s_i - x_i) \vec e_i$. For any such $\vec x$, the box $[\vec x, \vec s]\subseteq \mathcal M\cap\bar{\mathcal D}$ because if $\vec x' \ge \vec x$, then $F(\vec x', \vec r) \ge F(\vec x, \vec r) > \gamma_k$ and $G_i(\vec r, \vec x') \le G_i(\vec r, \vec x) \le 0$. Thus, also $\vec x^i = \vec s - (s_i - x_i) \vec e_i\in\mathcal M\cap\bar{\mathcal D}$.
Because $x_i \ge r_i$, we have $\vec x^i = \vec s - \alpha (s_i - r_i) \vec e_i$ for some $\alpha\in[0, 1]$. Since $\vec x^i \in \bar{\mathcal D}$, this and \cref{eq:reduction:alpha} implies $\alpha \le \alpha_i$. Hence, $\vec x^i \ge \vec r'$ and $\vec x \ge \vec r'$. Thus, every $\vec x\in\mathcal M\cap\mathcal D'$ is also in $\mathcal M'$ and, thus, $\mathcal M\cap\mathcal D' \subseteq \mathcal M'\cap\mathcal D'$.
The second reduction step in \cref{eq:reduction:s,eq:reduction:beta} can be proved analogously.
